# Supplementary material for: HACK3D: Crowdsourcing the Assessment of Cybersecurity in Digital Manufacturing
Source: arXiv:2005.04368 source file (2021-04-16)
Supplement: Supplementary file 1 [file appendix.tex]

\section*{Appendix: Hack3D Competitions}

Hack3D is a series of competitions organized by Center for Cybersecurity at New York University~\cite{hack3d}. It focuses on the security of additive manufacturing. We introduce details on the challenges and representative solutions submitted by the challenge participants as follows.

\subsection{Hack3D Challenge 1}

\begin{figure}[t] 
 \centering
 \includegraphics[width=0.9\columnwidth]{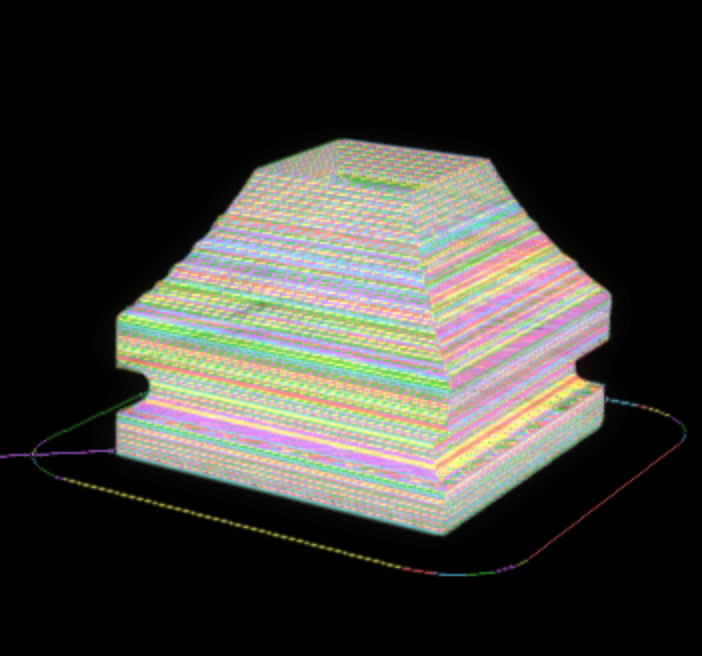}
 \caption{Damaged gcode file for Hack3D challenge 1.}
 \label{fig:chess_base}
\end{figure} 

\begin{figure}[t] 
 \centering
 \includegraphics[width=0.9\columnwidth]{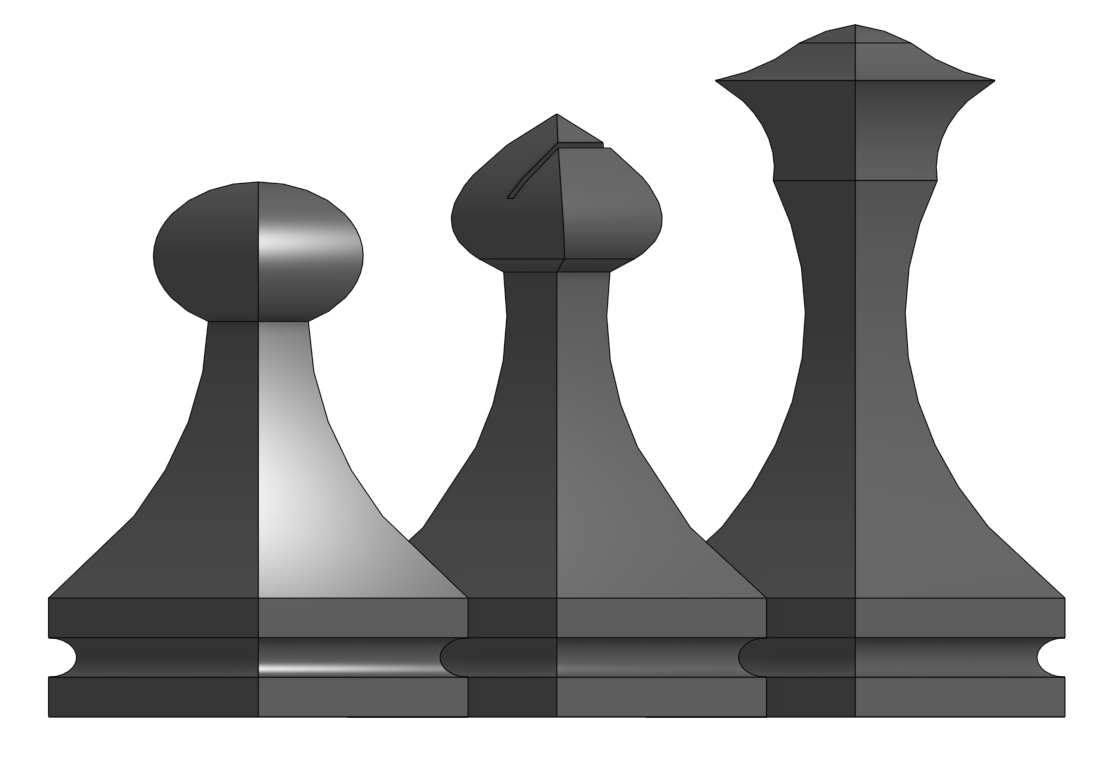}
 \caption{Three candidates for the damaged chess piece design.}
 \label{fig:chess_pieces}
\end{figure} 

The challenge participants are considered to be attackers who steal a partially damaged gcode file, which only models the bottom part of a chess piece, as opposed to a complete chess piece. Fig.~\ref{fig:chess_base} shows the damaged gcode as viewed in a gcode viewer. The participants need to solve two challenges: (1) among three candidates (Pawn, Bishop, and Queen), which chess piece is cut off in the damaged design, (2) the complete design of the piece. The challenge organizers also provide an orthographic image of all three candidates, as shown in Fig.~\ref{fig:chess_pieces}, and a text file with the true z-heights of each piece.

The challenge organizers also embedded a non-trivial shortcut in solving the challenge. They placed the design file of the top into a separate text file, which is stored on the cloud, giving view-only access to only those with a link. The link is embedded as a 3D QR code in the design of the chess base given to the participants. The challenge designers did not necessarily expect competitors to extract the hidden code in the chess piece in order to ``repair'' it. Unsurprisingly, some participants approached the challenge without reference to the 3D QR code within the chess model. The challenge participants demonstrated their creativity in attack methods. A few of the novel attacks are highlighted below. 

\vspace{2mm}
\noindent\textbf{Geometric Approach.} Making thorough use of information at hand, one of the teams was able to notice a discrepancy in the metadata of the G-code file. They realized that the filament to be used of the original piece (roughly 4290.7 mm) was different from that shown by their choice of G-Code viewer (roughly 3198.14 mm). They operated under the assumption that each of the pieces had a square cross-section.

Moreover, using the z-heights provided and extracting the height of the base piece from the G-code, they were able to tell where in the image the chess piece had been cut off. Hence, they cropped the tops off of each chess piece and used computer vision to measure the pixel dimensions, which they scaled using information from the G-code. In the end, they were able to produce G-code for the top of all three pieces. Since they knew the height difference between the original piece and the damaged piece, they were able to deduce that it was meant to be the queen top, as it matched closest in height. Their final result produced an error of 1\%. 

Another two teams processed the image and created a profile of the different chess piece edge, which produced a 1\% error in the geometry as the image processing led to a pixelated line. Based on this chess piece edge information, one of the teams created the shell of the queen with the help of a few reference points in the gcode and then filled the top and bottom layers with infill. The other team took a slightly different approach and produced a square prism at each point on the profile curve to recreate the pieces. Also, they figured that the chess piece was meant to be the queen based on the filament length information in the damaged gcode. 

\begin{figure}[t] 
 \centering
 \includegraphics[width=0.9\columnwidth]{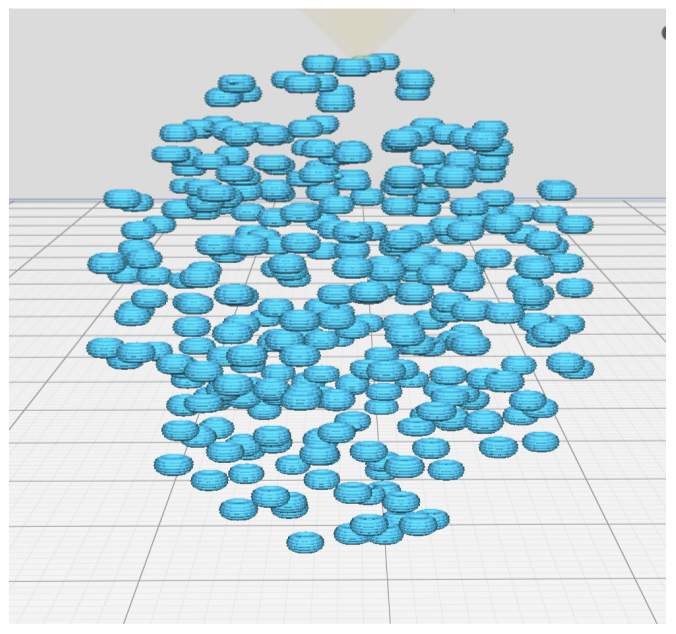}
 \caption{3D QR code viewed from a random direction.}
 \label{fig:spheres}
\end{figure} 

\begin{figure}[t] 
 \centering
 \includegraphics[width=0.9\columnwidth]{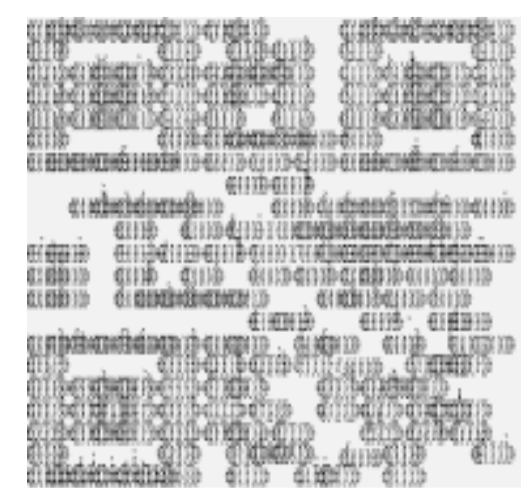}
 \caption{3D QR Code viewed from the correct direction.}
 \label{fig:qr_code}
\end{figure} 

\vspace{2mm}
\noindent\textbf{QR Code Extraction.} Two teams went down a route to look in the QR code embedded in the chess base. The QR code embedded is a bundle of spheres as shown in Fig.~\ref{fig:spheres}, and only when they are viewed from a certain direction, a QR code can be seen as Fig.~\ref{fig:qr_code}. One of the teams who attempted to extract the QR code was able to clean up the information in the gcode and extract a scannable code.

\subsection{Hack3D Challenge 2}

\begin{figure}[t] 
 \centering
 \includegraphics[width=0.9\columnwidth]{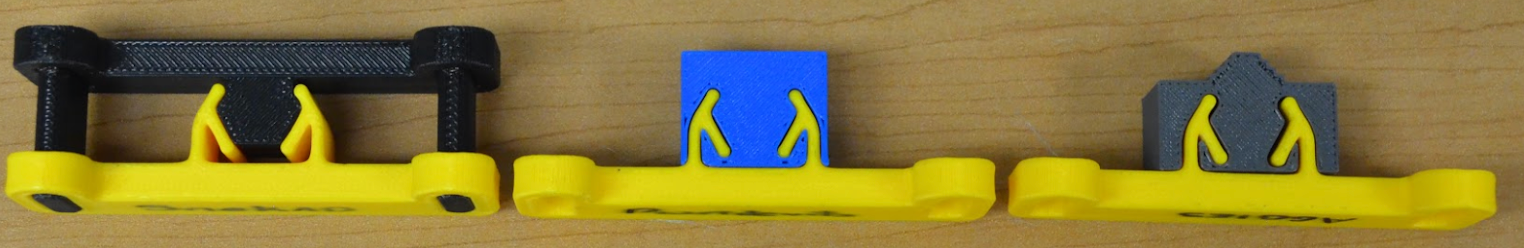}
 \caption{Solutions for Hack3D Challenge 2.}
 \label{fig:final_challenge}
\end{figure} 

In challenge 2, the competitors act as an attacker in a different phase. They are given a physical print, and a scaled-down version of STL file, instead of a gcode file, of a female connector (Fig.~\ref{fig:final_challenge}), and the challenge is to reconstruct the corresponding male connector. The specific focus is on the STL format and reverse engineering dimensions for compatibility. Similar to challenge 1, the design of the female connector has a 3D QR code embedded as well, which contains the password to an online server whose IP address and username are stored within the header data of the STL file. The design file of the corresponding male connector can be found in the server. %

Under a tight time constraint (6 hours), one team was able to extract the QR code to get the password, and they closely investigated the header of the given STL file. Thus, they were able to successfully retrieve the correct design file. Another team took a geometric approach and recreated a tight slide fit male part of the female part along with the scale factor. Although they were able to crack the QR code, they did not find the hidden message in the STL file, so they were not able to access the correct file stored in the server. Another unique attempt is made by another one of the final teams. While all other teams used CAD modeling software to reverse engineer the male part, this team abused the STL file directly and isolated a single cross-section of triangles to create a profile of the female part. After fine-tuning the profile, they created multiple iterations of a snug fit slide on the male connector. 

\subsection{Hack3D Challenge 3}

Hack3D challenge 3 gives the participants a set of XYZ coordinates in a 3D space, which describes the shape of a design (see Fig.~\ref{fig:hack3d_2018_target}). The participants have to use this information to recreate a 3D model of the object described by the XYZ coordinates. The XYZ coordinates can be visualized as a point cloud showed in Fig.~\ref{fig:hack3d_2018_point_cloud}.

The competitors used various tools (MeshLab, SolidWorks, OnShape) and self-developed Python scripts to reconstruct the point clouds, cross-sections, and eventually, the 3D model of the targeted design.

\begin{figure}[t] 
 \centering
 \includegraphics[width=0.9\columnwidth]{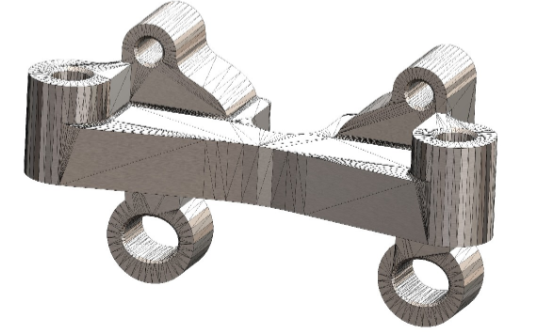}
 \caption{The Targeted Design of Hack3D Challenge 3.}
 \label{fig:hack3d_2018_target}
\end{figure} 

\begin{figure}[t] 
 \centering
 \includegraphics[width=0.9\columnwidth]{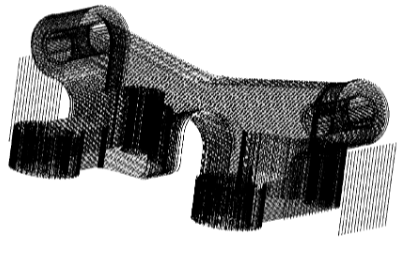}
 \caption{The Point Cloud Reconstructed from the XYZ Coordinates Given in Hack3D Challenge 3.}
 \label{fig:hack3d_2018_point_cloud}
\end{figure}
